# Supplementary material for: YouLeQD: Decoding the Cognitive Complexity of Questions and Engagement in Online Educational Videos from Learners' Perspectives
Source: arXiv:2501.11712 source file (2025-01-20)
Supplement: Supplementary file 1 [file appendix.tex]

\documentclass[conference]{IEEEtran}
\IEEEoverridecommandlockouts
%The preceding line is only needed to identify funding in the first footnote. If that is unneeded, please comment it out.
\usepackage{cite}
\usepackage{amsmath,amssymb,amsfonts}
\usepackage{algorithmic}
\usepackage{graphicx}
\usepackage{textcomp}
\usepackage{xcolor}
\usepackage{hyperref}
\usepackage{enumitem}
\usepackage{booktabs}
\usepackage{multirow, multicol}
\def\BibTeX{{\rm B\kern-.05em{\sc i\kern-.025em b}\kern-.08em
    T\kern-.1667em\lower.7ex\hbox{E}\kern-.125emX}}

\begin{document}

\title{Appendix}
\author{\IEEEauthorblockN{Anonymous Submission}
\IEEEauthorblockA{}
}

\maketitle

\end{document}
